# Supplementary material for: Graph Convolutional Matrix Completion
Source: arXiv:1706.02263 source file (2017-10-25)
Supplement: Supplementary file 1 [file appendix.tex]

\section{Appendix}
